# Supplementary material for: Towards Efficient Integration of Blockchain for IoT Security: The Case Study of IoT Remote Access
Source: arXiv:1912.00264 source file (2019-11-30)
Supplement: Supplementary file 1 [file appendix.tex]

\appendix
\section{APPENDIX}
\subsection{Mirai \& its Variants}\label{sec:variant}
\subsubsection{Miari Botnet}
The IoT oriented botnet malware 'Mirai' spread from September 2016 had caused record-breaking DDoS with traffic flow of over 660 Gbps. Soon after that the source code of Mirai was published and can be publicly accessed on Github \cite{mirai_source}. According to the publicized source code, there are about 60 hardcoded default telnet username password pairs that are used to log into the victim hosts. With a successful login, the attacker load the executable malware execute it. After that, the compromised device joins the bot army by scanning potential victims and reporting login credentials to botnet master server. After infection, the malware would delete the executable binary from device storage while shutdown all accessible network ports for protecting itself. Though Mirai is still a coarse botnet malware without DGA (domain generation algorithm) or P2P network to hide the location of C\&C server, the release of its source code inspires other imitators to create much more sophisticated variants.

\subsubsection{Hajime Bot\cite{hajime}}
Hajime \cite{Hajime_detail} is the first Mirai variant that was found Oct 5, 2016. Unlike equipping with the centralized malware loader as Mirai, Hajime utilized the P2P network to load the malware which makes the analysis of it much more difficult. It uses the same scanning and brute-force cracking attack method as Mirai uses \cite{mirai_source}. The difference is it utilizes the P2P network to push message to the bot nodes instead have hardcoded command and control server's domain name inside the source code. Besides, Hajime is a modulized malware, and the author keeps on developing new modules like CPU architecture support and UPnP IGD vulnerability exploitation to enforce the malware's capability.

\subsubsection{Satori/Okiru Bot}
This Mirai variant is discovered in late November 2017 and targeting the Huawei's router HG532. The Satori exploits one old vulnerability (CVE-2014-8316) and one zero-day vulnerability (CVE-2017-17215) to take down target device. All these vulnerabilities are related to command injection in UPnP SOAP interface. The vulnerability is located at UPnP IGD (Internet Gateway Device) Implementation \cite{Huawei_upnp}. In the implementation, the AddPortMapping service is mistakenly exposed to the Internet. This allows attackers to inject command at the \textbf{NewInternetClient} parameter. 

\subsubsection{Masuta/PureMasuta}
Masuta\cite{HNAP_exploitation} is a newly emerged Mirai variant produced by the same author of Satori. This variant takes advantage of D-Link's HNAP (Home Network Administration Protocol) software as its weapon. HNAP is also a SOAP (Simple Object Access Protocol) based protocol for network admins to manage the network devices. This protocol, published by PureNetwork (acquired by Cisco), is reported to have a vulnerability in 2015. However, it's still left unpatched by the date of attack happened.  In summary, this vulnerability allows attackers to get the router's login name and password remotely by sending forged HTTP GET request. Combined with the remote command execution (RCE) vulnerability in device common gateway interface (CGI), attackers can remotely log into the victim devices with root privilege and execute arbitrary codes.

\subsubsection{Deutsche Telekom Bot (TR-069 abuse)}
This kind of botnet was first detected in November 2016. It manipulates the CPE WAN Management Protocol (CWMP), an HTTP-based protocol that enables auto-configuration and remote management of home routers, modems, and other customer premises equipment (CPE). This exploit led to an out-age at Deutsche Telekom late November 2016

\subsubsection{ZyXEL Default Password}
This Mirai variant is noticed in November 2017 by 360 secure Netlab\cite{zyxel}. It's discovered by the detection of large scanning traffic on port 23/2323 by over 100k scanner IP from Argentina. During this attack,two new default credentials been used by this malware: \textbf{admin/CenturyLink} and \textbf{admin/QwestModem}. 

ZyXEL is a Taiwanese router manufacturer; its product is reported to have vulnerability on administration login process that can let attackers bypass the authentication (CVE-2017-3216 \cite{CVE_bypass}) in June 2017. After that, some other vulnerabilities are found on its products including backdoor telnet with default password, CGI command injection (CVE-2017-(7964,6884,15226,17901)). ZyXEL hasn't finished patching up all these flaws and just advised users disable the WAN management access on their router which is enabled by default.

\subsubsection{Summary}
From the retrospection of Mirai and its variants, we can find some shared characters
\begin{itemize}
    \item Employ bot nodes to scan random IP addresses
    \item Exploits application-level software vulnerabilities
    \item Home routers make up the largest portion of the victim device type. 
\end{itemize}

These common characters trend revealed the fact that one important prerequisite for IoT botnet's propagation is the victim device can be accessed directly from the Internet. Explicitly, routers bear the brunt of the malware as most of them serve as the gateway with public IP address. In Mirai botnet attack, compromised NVR and IP cameras which should usually reside behind the Network Address Translation (NAT) shield of home routers are exposed by the use of UPnP IGD protocol which does port mapping automatically to enable user remote access. Although UPnP-IGD is considered as dangerous long before the botnet attack, a lot of home router products still get this function enabled by default.  After the reap of Mirai, most vulnerable UPnP devices are infected and no longer accessible from the Internet, while others may have disabled the port mapping feature and turn to the cloud relay method for remote accessing as we'll discuss in section\ref{sec:cur}. As a result, the only target left for botnet malware is the home router which is inevitably exposed on the public Internet.

\subsection{Smart Contract Background}
The concept of smart contract is introduced by Vitalik Buterin \cite{buterin2014next} in 2013. In Ethereum whitepaper \cite{buterin2014next}, the smart contract is described as script code implemented on Blockchain to deal with digital assets. Different from prior Bitcoin script, the general computing platform is achieved in Ethereum contract by enabling turning complete functions. Smart contract bytecode derived from high-level script languages are executed in an isolated environment which is called as Ethereum Virtual Machine (EVM). Smart contract platform can be regarded as a global computer where, in theory, all nodes will execute the contract code and then reach consensus on execution results, and incorrect execution with wrong results would be discarded by other nodes in the blockchain network and thus be excluded from the main chain. The verification of execution result conducted during consensus procedures gives the Ethereum global computer the feature of trusted computing and tampering resistance. 

In Ethereum platform, two types of account are provided:1) personal account is set up by individual users for launching ether transfer or interacting with contract functions, and it's protected by personal private key; 2) Contract account is the location of contract code whose security is ensured by the aforementioned trusted contract execution. Both two types of accounts can store a balance of cryptocurrency. To prevent the computing power of the "global computer" be maliciously occupied and remunerate miners who execute the contract code, each operation of the contract code has associated processing fee calculated in "gas" which is dynamically pegged with current digital asset unit "Ether". Although the execution of contract code is not free, it provides following favorable features:
\begin{itemize}
    \item The execution of the contract is deterministic that can be verified by any node at any time after the execution
    \item The result of execution is tampering resistance and nondeniable
    \item Correctness of contract execution is ensured
\end{itemize}
In our work, smart contract serves as the arbiter in relay sharing platform to guarantee fairness in service trading and execute punishment on misbehavior.
